# Supplementary material for: Private, Verifiable, and Auditable AI Systems
Source: arXiv:2509.00085 source file (2025-08-27)
Supplement: Supplementary file 1 [file appendixa.tex]

% From mitthesis package
% Version: 1.01, 2023/07/04
% Documentation: https://ctan.org/pkg/mitthesis
