# Supplementary material for: Private, Verifiable, and Auditable AI Systems
Source: arXiv:2509.00085 source file (2025-08-27)
Supplement: Supplementary file 2 [file biography.tex]

%% biography.tex
%% This section is optional

% From mitthesis package
% Version: 1.02, 2024/06/19
% Documentation: https://ctan.org/pkg/mitthesis

\chapter*{Biographical Sketch}
\pdfbookmark[0]{Biographical Sketch}{biosketch}

Silas Whitcomb Holman was born in Harvard, Massachusetts on January 20, 1856. He received his S.B. degree in Physics from MIT in 1876, and then joined the MIT Department of Physics as an Assistant. He became Instructor in Physics in 1880, Assistant Professor in 1882, Associate Professor in 1885, and Full Professor in 1893. Throughout this period, he struggled with increasingly severe rheumatoid arthritis. At length, he was defeated, becoming Professor Emeritus in 1897 and dying on April 1, 1900.

Holman's light burned brilliantly before his tragic and untimely death. He published extensively in thermal physics, and authored textbooks on precision measurement, fundamental mechanics, and other subjects. He established the original Heat Measurements Laboratory. Holman was a much admired teacher among both his students and his colleagues. The reports of his department and of the Institute itself refer to him frequently in the 1880's and 1890's, in tones that gradually shift from the greatest respect to the deepest sympathy.

Holman was a student of Professor Edward C. Pickering, then head of the Physics department. Holman himself became second in command of Physics, under Professor Charles R. Cross, some years later. Among Holman's students, several went on to distinguish themselves, including: the astronomer George E. Hale ('90) who organized the Yerkes and Mt. Wilson observatories and who designed the 200 inch telescope on Mt. Palomar; Charles G. Abbot ('94), also an astrophysicist and later Secretary of the Smithsonian Institution; and George K. Burgess ('96), later Director of the Bureau of Standards.
